# Supplementary material for: Interim Analysis in Sequential Multiple Assignment Randomized Trials for Survival Outcomes
Source: arXiv:2504.03143 source file (2025-04-04)
Supplement: Supplementary file 1 [file SM_Biometrics.pdf]

**Supplementary Material for “Interim Analysis in Sequential Multiple  
Assignment Randomized Trials for Survival Outcomes” by Zi Wang, Yu Cheng,  
and A.S. Wahed**

**Zi Wang<sup>1,\*</sup>, Yu Cheng<sup>1,\*\*</sup>, and Abdus, S. Wahed<sup>2,\*\*\*</sup>**

<sup>1</sup>Department of Statistics, University of Pittsburgh, Pittsburgh, Pennsylvania, U.S.A.

<sup>2</sup>Department of Biostatistics and Computational Biology, University of Rochester, Rochester, New York, U.S.A.

*\*email: ziw43@pitt.edu*

*\*\*email: yucheng@pitt.edu*

*\*\*\*email: abdus\_wahed@urmc.rochester.edu*

## Web Appendix A. Additional Simulation Results

Table 1 summarizes true parameter values under various simulation studies. In Section 4, we evaluate the weighted log-rank and Tsiatis and Davidian’s statistics under 20% censoring rate with a second-stage entry proportion of  $p_\eta = 0.9$  and  $n = 500$ . Web Tables 2 and 3 show the performance of the statistics with censoring rate of 10% and 40% under null scenarios. Consistent with what we’ve seen in Table 2 of the main manuscript, the type I errors from the bootstrapped estimator are generally inflated. Web Tables 2 and 3 show that higher censoring rates tend to result in slightly lower type I errors, making the decision more conservative. We observe similar trends when  $p_\eta = 0.75$  of individuals enter the second stage with 10%, 20%, and 40% censoring in Web Tables 4, 5 and 6.

Next, we evaluate power under four alternatives (Alt 1-Alt 4) with 10% (Table 7) and 20% censoring (Table 3 of the main manuscript). Not surprisingly, we observe decreasing power with increasing censoring. When we increase the censoring rate to 40%, power is further reduced. We only present the power for Alt 1 and Alt 3 in Web Table 8 (Alt 2 and Alt 4 are similar and omitted here), but under two different sample sizes  $n = 500$  and  $n = 1000$ . Increasing the sample size improves the tests’ power, leading to a greater reduction in required sample size through interim monitoring. When we lower  $p_\eta$  to 75%, we observe slightly decreased power, by comparing Web Table 7 to Web Table 9 for 10% censoring, and Web Table 10 for 20% censoring.

[Web Table 1 about here.]

[Web Table 2 about here.]

[Web Table 3 about here.]

[Web Table 4 about here.]

[Web Table 5 about here.]

[Web Table 6 about here.]

[Web Table 7 about here.]

[Web Table 8 about here.]

[Web Table 9 about here.]

[Web Table 10 about here.]

**Web Appendix B. Additional table for the neuroblastoma study**

Web Table 11 presents the estimated Pocock (Pocock, 1977), O’Brien-Fleming (OBF) (O’Brien and Fleming, 1979), and Lan-DeMets (Lan and Demets, 1983) efficacy boundaries for the neuroblastoma data. The web table indicates that the calculated boundaries for the the weighted log-rank and Tsiatis and Davidian’s estimators are similar.

[Web Table 11 about here.]

## References

- Lan, K. and Demets, D. L. (1983). Discrete sequential boundaries for clinical trials. *Biometrics* **70**, 659–663.
- O’Brien, P. C. and Fleming, T. R. (1979). A multiple testing procedure for clinical trials. *Biometrics* **35**, 549–556.
- Pocock, S. J. (1977). Group sequential methods in the design and analysis of clinical trials. *Biometrika* **64**, 191–199.
- Tsiatis, A. A. and Davidian, M. (2024). A generalized logrank-type test for comparison of treatment regimes in sequential multiple assignment randomized trials. *Biometrics*. *arXiv preprint arXiv:2403.16813* .

Table 1: Details of the null and alternative scenarios. Parameters are described in Section 4.1

| Scenario                                               | Null   |        | Alt      |            |          |          |
|--------------------------------------------------------|--------|--------|----------|------------|----------|----------|
| Design                                                 | SMART1 | SMART2 | SMART1   |            | SMART2   |          |
| Parameter                                              | Null1  | Null2  | Alt1     | Alt2       | Alt3     | Alt4     |
| $\theta_1^N$                                           | 5      | 3      | 5        | 5          | 3        | 3        |
| $\theta_2^N$                                           | 5      | 3      | 5        | 5          | 3        | 3        |
| $\theta_1$                                             | 5      | 3      | 5        | 5          | 3        | 3        |
| $\theta_2$                                             | 5      | 3      | 5        | 5          | 3        | 3        |
| $(\theta_{11}^R, \theta_{12}^R)$                       | (5, 5) | (2, 2) | (2, 4)   | (2.8, 4.6) | (2, 3.2) | (2.7, 6) |
| $(\theta_{21}^R, \theta_{22}^R)$                       | (5, 5) | (2, 2) | (3, 4)   | (2.3, 4.9) | (2.5, 4) | (4.9, 3) |
| $(\theta_{11}^{NR}, \theta_{12}^{NR}) / \theta_1^{NR}$ | (5, 5) | 5      | (3.2, 3) | (5.8, 4.3) | 6        | 3.8      |
| $(\theta_{21}^{NR}, \theta_{22}^{NR}) / \theta_2^{NR}$ | (5, 5) | 5      | (2.9, 2) | (5.2, 6.5) | 6        | 7.2      |
| $\nu$ (10% censoring rate)                             | 3.8    | 5.8    | 4.9      | 4.3        | 5.8      | 5.5      |
| $\nu$ (20% censoring rate)                             | 1.9    | 2.9    | 2.5      | 2.1        | 2.9      | 2.8      |
| $\nu$ (40% censoring rate)                             | 0.9    | 1.6    | 1.2      | 1.0        | 1.4      | 1.3      |

Table 2: Simulation results for two SMART designs under Null Scenarios with censoring rate around 10%

| M | Boundary  | Rejection Rate | SMART1 |     |     |     | SMART2 |      |     |      |
|---|-----------|----------------|--------|-----|-----|-----|--------|------|-----|------|
|   |           |                | LR     | BLR | TD  | BTD | LR     | BLR  | TD  | BTD  |
| 1 | NA        | Power          | 4.3    | 4.9 | 7.2 | 7.5 | 5.6    | 9.0  | 6.2 | 9.2  |
|   | Oracle    | Rej at interim | 2.2    | 2.4 | 4.6 | 5.9 | 3.3    | 6.8  | 4.0 | 7.3  |
|   |           | Rej at final   | 1.7    | 2.5 | 2.8 | 4.0 | 2.5    | 4.5  | 2.6 | 4.9  |
|   |           | Type I Error   | 4.0    | 4.9 | 7.3 | 9.8 | 5.8    | 11.0 | 6.5 | 11.9 |
|   | OBF       | Rej at interim | 0.7    | 0.4 | 2.1 | 2.1 | 2.0    | 3.3  | 2.0 | 3.2  |
|   |           | Rej at final   | 4.5    | 4.4 | 5.8 | 6.3 | 4.1    | 7.5  | 4.5 | 7.3  |
|   |           | Type I Error   | 5.2    | 4.9 | 7.8 | 8.3 | 6.0    | 10.6 | 6.5 | 10.9 |
|   | Pocock    | Rej at interim | 2.1    | 2.9 | 4.2 | 5.7 | 3.0    | 5.6  | 3.9 | 6.5  |
|   |           | Rej at final   | 1.7    | 2.2 | 2.6 | 3.6 | 2.1    | 3.8  | 2.3 | 4.1  |
|   |           | Type I Error   | 3.8    | 5.0 | 6.7 | 9.2 | 5.1    | 9.2  | 6.2 | 10.4 |
|   | OBF       | Rej at interim | 0.2    | 0.4 | 2.2 | 2.2 | 1.6    | 3.7  | 2.1 | 3.5  |
|   |           | Rej at final   | 4.3    | 4.7 | 6.5 | 6.7 | 5.3    | 8.0  | 5.2 | 7.9  |
|   |           | Type I Error   | 4.5    | 5.1 | 8.6 | 8.8 | 6.9    | 11.4 | 7.2 | 11.2 |
|   | LD-Pocock | Rej at interim | 2.8    | 2.7 | 4.8 | 6.3 | 2.4    | 2.6  | 4.2 | 7.8  |
|   |           | Rej at final   | 1.5    | 2.1 | 2.6 | 3.8 | 2.8    | 8.0  | 2.4 | 4.2  |
|   |           | Type I Error   | 4.3    | 4.7 | 7.3 | 9.9 | 5.2    | 10.4 | 6.5 | 11.7 |
| 2 | LD-OBF    | Rej at interim | 0.1    | 0.4 | 2.0 | 2.0 | 1.4    | 7.6  | 1.6 | 2.0  |
|   |           | Rej at final   | 4.1    | 4.4 | 5.8 | 6.6 | 4.5    | 4.0  | 4.9 | 7.6  |
|   |           | Type I Error   | 4.2    | 4.8 | 7.7 | 8.5 | 5.9    | 11.3 | 6.5 | 9.5  |

M: Number of total analysis including the final. Rej at interim: rejection rate at the interim analysis. Rej at final: the probability of rejection at the final analysis condition on not rejecting at the interim analysis. Oracle: boundaries calculated using full data at interim. LR and TD: the proposed weighted log-rank and Tsiatis and Davidian (2024) statistics normalized using the proposed covariance estimates. BLR and BTD: the statistics normalized using the bootstrap covariance estimates. LD-Pocock and LD-OBF: Pocock and OBF boundaries obtained using a particular error spending function recommended by Lan and Demets (1983). Results are shown in percentages within 1 decimal place.

Table 3: Simulation results for two SMART designs under Null Scenario with censoring rate around 40%

| M | Boundary  | Rejection Rate | SMART1 |     |     |     | SMART2 |     |     |     |
|---|-----------|----------------|--------|-----|-----|-----|--------|-----|-----|-----|
|   |           |                | LR     | BLR | TD  | BTD | LR     | BLR | TD  | BTD |
| 1 | NA        | Power          | 3.7    | 4.4 | 4.7 | 6.6 | 4.5    | 8.0 | 4.6 | 7.7 |
| 2 | Oracle    | Rej at interim | 1.3    | 3.2 | 3.4 | 5.0 | 2.8    | 6.3 | 2.8 | 5.9 |
|   |           | Rej at final   | 2.2    | 2.0 | 1.9 | 3.2 | 1.6    | 3.8 | 1.6 | 3.5 |
|   |           | Type I Error   | 3.5    | 5.2 | 5.2 | 8.1 | 4.4    | 9.9 | 4.4 | 9.2 |
|   | Pocock    | Rej at interim | 0.1    | 0.9 | 1.2 | 2.3 | 0.7    | 2.3 | 0.8 | 2.5 |
|   |           | Rej at final   | 3.5    | 3.9 | 4.3 | 5.6 | 3.4    | 6.5 | 3.5 | 6.3 |
|   |           | Type I Error   | 3.6    | 4.8 | 5.4 | 7.8 | 4.1    | 8.7 | 4.3 | 8.7 |
|   | Oracle    | Rej at interim | 1.1    | 3.1 | 3.0 | 4.9 | 2.7    | 5.4 | 2.5 | 4.6 |
|   |           | Rej at final   | 2.1    | 2.0 | 1.8 | 3.1 | 1.6    | 3.4 | 1.3 | 3.1 |
|   |           | Type I Error   | 3.2    | 5.1 | 4.7 | 7.9 | 4.3    | 8.7 | 3.8 | 7.6 |
|   | OBF       | Rej at interim | 0.1    | 0.9 | 1.3 | 2.3 | 1.1    | 2.8 | 1.0 | 2.6 |
|   |           | Rej at final   | 3.7    | 4.1 | 4.3 | 5.8 | 4.0    | 7.3 | 3.8 | 7.0 |
|   |           | Type I Error   | 3.8    | 5.0 | 5.5 | 8.0 | 5.1    | 9.9 | 4.8 | 9.4 |
|   | LD-Pocock | Rej at interim | 2.0    | 3.5 | 3.5 | 5.5 | 3.1    | 1.8 | 3.2 | 6.1 |
|   |           | Rej at final   | 1.4    | 1.7 | 1.7 | 2.9 | 1.4    | 7.1 | 1.4 | 3.2 |
|   |           | Type I Error   | 3.4    | 5.2 | 5.1 | 8.3 | 4.5    | 8.8 | 4.6 | 9.1 |
|   | LD-OBF    | Rej at interim | 0.3    | 0.9 | 0.9 | 2.1 | 0.5    | 6.8 | 0.6 | 1.5 |
|   |           | Rej at final   | 2.9    | 3.9 | 4.4 | 5.7 | 3.8    | 3.3 | 3.8 | 6.9 |
|   |           | Type I Error   | 3.2    | 4.8 | 5.3 | 7.7 | 4.3    | 9.9 | 4.4 | 8.3 |

M: Number of total analysis including the final. Rej at interim: rejection rate at the interim analysis. Rej at final: the probability of rejection at the final analysis condition on not rejecting at the interim analysis. Oracle: boundaries calculated using full data at interim. LR and TD: the proposed weighted log-rank and Tsiatis and Davidian (2024) statistics normalized using the proposed covariance estimates. BLR and BTD: the statistics normalized using the bootstrap covariance estimates. LD-Pocock and LD-OBF: Pocock and OBF boundaries obtained using a particular error spending function recommended by Lan and Demets (1983). Results are shown in percentages within 1 decimal place.



Table 4: Simulation results for two SMART designs under Null Scenarios with  $p_\eta = 0.75$  (censoring rate:10%)

| M | Boundary  | Rejection Rate | SMART1 |     |     |      | SMART2 |     |     |     |
|---|-----------|----------------|--------|-----|-----|------|--------|-----|-----|-----|
|   |           |                | LR     | BLR | TD  | BTD  | LR     | BLR | TD  | BTD |
| 1 | NA        | Type I Error   | 5.3    | 4.6 | 7.6 | 10.5 | 5.3    | 7.5 | 5.4 | 7.8 |
|   | Oracle    | Rej at interim | 2.7    | 2.9 | 4.3 | 5.5  | 4.4    | 4.5 | 4.1 | 4.5 |
|   |           | Rej at final   | 2.7    | 2.6 | 4.2 | 5.1  | 1.8    | 3.7 | 1.8 | 3.2 |
|   |           | Type I Error   | 5.3    | 5.4 | 8.3 | 10.4 | 6.1    | 8.0 | 5.8 | 7.6 |
|   | Pocock    | Rej at interim | 0.2    | 0.6 | 1.3 | 2.2  | 1.7    | 1.8 | 1.1 | 1.8 |
|   |           | Rej at final   | 5.1    | 4.4 | 6.7 | 9.5  | 3.9    | 6.0 | 4.4 | 6.4 |
|   |           | Type I Error   | 5.3    | 5.0 | 7.9 | 11.5 | 5.5    | 7.7 | 5.5 | 8.1 |
|   | Oracle    | Rej at interim | 2.2    | 2.4 | 4.9 | 4.6  | 3.8    | 3.8 | 3.5 | 4.1 |
|   |           | Rej at final   | 2.6    | 2.2 | 3.0 | 4.7  | 1.8    | 3.1 | 1.5 | 2.6 |
|   |           | Type I Error   | 4.7    | 4.5 | 7.8 | 9.1  | 5.5    | 6.8 | 4.9 | 6.6 |
|   | OBF       | Rej at interim | 0.5    | 0.6 | 1.3 | 2.2  | 1.9    | 2.1 | 1.7 | 1.9 |
|   |           | Rej at final   | 5.2    | 4.8 | 7.0 | 10.0 | 4.4    | 6.3 | 4.5 | 6.8 |
|   |           | Type I Error   | 5.7    | 5.4 | 8.2 | 12.0 | 6.2    | 8.3 | 6.1 | 8.6 |
|   | Pocock    | Rej at interim | 2.8    | 3.1 | 4.5 | 5.9  | 4.4    | 4.8 | 4.8 | 4.9 |
|   |           | Rej at final   | 2.3    | 1.8 | 3.7 | 4.9  | 1.8    | 3.5 | 1.5 | 2.4 |
|   |           | Type I Error   | 5.0    | 4.8 | 8.0 | 10.5 | 6.1    | 8.1 | 6.2 | 7.2 |
| 2 | LD-Pocock | Rej at interim | 0.3    | 0.6 | 1.0 | 2.0  | 0.8    | 1.2 | 0.6 | 1.3 |
|   |           | Rej at final   | 5.1    | 4.4 | 7.1 | 10.0 | 4.6    | 6.7 | 4.9 | 6.8 |
|   |           | Type I Error   | 5.4    | 5.0 | 8.0 | 11.8 | 5.4    | 7.8 | 5.5 | 8.0 |
|   | LD-OBF    | Rej at interim | 0.3    | 0.6 | 1.0 | 2.0  | 0.8    | 1.2 | 0.6 | 1.3 |
|   |           | Rej at final   | 5.1    | 4.4 | 7.1 | 10.0 | 4.6    | 6.7 | 4.9 | 6.8 |
|   |           | Type I Error   | 5.4    | 5.0 | 8.0 | 11.8 | 5.4    | 7.8 | 5.5 | 8.0 |

M: Number of total analysis including the final. Rej at interim: rejection rate at the interim analysis. Rej at final: the probability of rejection at the final analysis condition on not rejecting at the interim analysis. Oracle: boundaries calculated using full data at interim. LR and TD: the proposed weighted log-rank and Tsiatis and Davidian (2024) statistics normalized using the proposed covariance estimates. BLR and BTD: the statistics normalized using the bootstrap covariance estimates. LD-Pocock and LD-OBF: Pocock and OBF boundaries obtained using a particular error spending function recommended by Lan and Demets (1983). Results are shown in percentages within 1 decimal place.

Table 5: Simulation results for two SMART designs under Null Scenarios with  $p_\eta = 0.75$  (censoring rate:20%)

| M | Boundary  | Rejection Rate | SMART1 |     |     |      | SMART2 |     |     |     |
|---|-----------|----------------|--------|-----|-----|------|--------|-----|-----|-----|
|   |           |                | LR     | BLR | TD  | BTD  | LR     | BLR | TD  | BTD |
| 1 | NA        | Type I Error   | 5.5    | 5.8 | 7.3 | 11.2 | 4.8    | 7.3 | 4.3 | 7.6 |
|   | Oracle    | Rej at interim | 2.2    | 3.3 | 4.5 | 6.6  | 4.6    | 3.8 | 4.3 | 4.2 |
|   |           | Rej at final   | 2.5    | 2.5 | 2.8 | 5.9  | 1.6    | 4.2 | 1.9 | 3.5 |
|   |           | Type I Error   | 4.7    | 5.8 | 7.2 | 12.1 | 6.2    | 7.8 | 6.2 | 7.6 |
|   | Pocock    | Rej at interim | 0.5    | 0.8 | 2.2 | 1.8  | 1.6    | 2.0 | 1.4 | 2.4 |
|   |           | Rej at final   | 4.5    | 5.0 | 6.2 | 10.0 | 3.6    | 5.8 | 3.4 | 6.0 |
|   |           | Type I Error   | 5.0    | 5.8 | 8.3 | 11.6 | 5.1    | 7.7 | 4.8 | 8.3 |
|   | Oracle    | Rej at interim | 2.2    | 3.3 | 4.3 | 5.9  | 3.9    | 3.5 | 3.9 | 3.8 |
|   |           | Rej at final   | 2.5    | 2.4 | 2.7 | 5.6  | 1.9    | 3.6 | 1.7 | 3.2 |
|   |           | Type I Error   | 4.6    | 5.7 | 6.9 | 11.2 | 5.7    | 7.0 | 5.6 | 6.9 |
|   | OBF       | Rej at interim | 0.6    | 0.8 | 2.2 | 2.1  | 2.0    | 2.2 | 1.7 | 2.5 |
|   |           | Rej at final   | 5.2    | 5.4 | 6.7 | 10.8 | 3.6    | 6.4 | 3.3 | 6.7 |
|   |           | Type I Error   | 5.8    | 6.2 | 8.8 | 12.7 | 5.6    | 8.5 | 5.0 | 9.0 |
| 2 | Pocock    | Rej at interim | 2.6    | 3.5 | 5.0 | 7.2  | 4.9    | 3.9 | 4.6 | 4.2 |
|   |           | Rej at final   | 2.4    | 2.5 | 2.7 | 5.2  | 1.4    | 3.7 | 1.6 | 3.4 |
|   |           | Type I Error   | 4.9    | 5.9 | 7.6 | 12.0 | 6.3    | 7.5 | 6.2 | 7.6 |
|   | LD-Pocock | Rej at interim | 0.5    | 0.8 | 2.0 | 1.5  | 0.7    | 1.5 | 0.7 | 1.6 |
|   |           | Rej at final   | 4.5    | 5.0 | 6.3 | 10.2 | 3.9    | 6.3 | 3.6 | 6.6 |
|   |           | Type I Error   | 5.0    | 5.8 | 8.2 | 11.6 | 4.6    | 7.7 | 4.3 | 8.1 |
|   | LD-OBF    | Rej at interim | 0.5    | 0.8 | 2.0 | 1.5  | 0.7    | 1.5 | 0.7 | 1.6 |
|   |           | Rej at final   | 4.5    | 5.0 | 6.3 | 10.2 | 3.9    | 6.3 | 3.6 | 6.6 |
|   |           | Type I Error   | 5.0    | 5.8 | 8.2 | 11.6 | 4.6    | 7.7 | 4.3 | 8.1 |

M: Number of total analysis including the final. Rej at interim: rejection rate at the interim analysis. Rej at final: the probability of rejection at the final analysis condition on not rejecting at the interim analysis. Oracle: boundaries calculated using full data at interim. LR and TD: the proposed weighted log-rank and Tsiatis and Davidian (2024) statistics normalized using the proposed covariance estimates. BLR and BTD: the statistics normalized using the bootstrap covariance estimates. LD-Pocock and LD-OBF: Pocock and OBF boundaries obtained using a particular error spending function recommended by Lan and Demets (1983). Results are shown in percentages within 1 decimal place.

Table 6: Simulation results for two SMART designs under Null Scenarios with  $p_\eta = 0.75$  (censoring rate:40%)

| M | Boundary  | Rejection Rate | SMART1 |     |     |      | SMART2 |     |     |     |
|---|-----------|----------------|--------|-----|-----|------|--------|-----|-----|-----|
|   |           |                | LR     | BLR | TD  | BTD  | LR     | BLR | TD  | BTD |
| 1 | NA        | Type I Error   | 5.0    | 6.0 | 5.9 | 8.9  | 4.6    | 6.3 | 4.4 | 6.6 |
|   | Oracle    | Rej at interim | 1.8    | 2.3 | 2.2 | 4.8  | 2.6    | 3.8 | 2.3 | 3.5 |
|   |           | Rej at final   | 2.0    | 2.8 | 3.7 | 5.9  | 2.6    | 3.6 | 2.7 | 3.5 |
|   |           | Type I Error   | 3.8    | 6.0 | 5.8 | 10.4 | 5.1    | 7.3 | 4.9 | 6.9 |
|   | Pocock    | Rej at interim | 0.3    | 0.7 | 0.4 | 1.4  | 1.3    | 1.3 | 1.3 | 1.2 |
|   |           | Rej at final   | 4.6    | 5.5 | 5.4 | 8.4  | 4.1    | 5.3 | 3.7 | 5.5 |
|   |           | Type I Error   | 4.9    | 6.2 | 5.8 | 9.7  | 5.3    | 6.5 | 5.0 | 6.6 |
|   | Oracle    | Rej at interim | 1.7    | 2.2 | 2.0 | 4.0  | 2.2    | 3.3 | 1.9 | 3.0 |
|   |           | Rej at final   | 1.9    | 3.4 | 3.2 | 5.8  | 2.2    | 3.4 | 2.4 | 3.2 |
|   |           | Type I Error   | 3.6    | 5.5 | 5.1 | 9.6  | 4.4    | 6.6 | 4.3 | 6.1 |
|   | OBF       | Rej at interim | 0.3    | 0.7 | 0.4 | 1.4  | 1.3    | 1.6 | 1.5 | 1.7 |
|   |           | Rej at final   | 4.7    | 6.0 | 5.6 | 8.8  | 4.3    | 5.7 | 4.2 | 5.8 |
|   |           | Type I Error   | 5.0    | 6.7 | 6.0 | 10.1 | 5.6    | 7.2 | 5.6 | 7.4 |
|   | Pocock    | Rej at interim | 1.9    | 2.5 | 2.5 | 5.3  | 2.7    | 3.8 | 2.7 | 3.6 |
|   |           | Rej at final   | 1.9    | 3.1 | 3.5 | 5.5  | 2.4    | 3.4 | 2.6 | 3.3 |
|   |           | Type I Error   | 3.8    | 5.6 | 5.9 | 10.5 | 5.0    | 7.1 | 5.2 | 6.8 |
| 2 | LD-Pocock | Rej at interim | 0.3    | 0.7 | 0.4 | 1.3  | 0.7    | 0.9 | 0.8 | 0.7 |
|   |           | Rej at final   | 4.6    | 5.5 | 5.6 | 8.7  | 4.2    | 5.8 | 4.3 | 5.7 |
|   |           | Type I Error   | 4.9    | 6.2 | 6.0 | 9.9  | 4.9    | 6.6 | 5.1 | 6.4 |
|   | LD-OBF    | Rej at interim | 0.3    | 0.7 | 0.4 | 1.3  | 0.7    | 0.9 | 0.8 | 0.7 |
|   |           | Rej at final   | 4.6    | 5.5 | 5.6 | 8.7  | 4.2    | 5.8 | 4.3 | 5.7 |
|   |           | Type I Error   | 4.9    | 6.2 | 6.0 | 9.9  | 4.9    | 6.6 | 5.1 | 6.4 |

M: Number of total analysis including the final. Rej at interim: rejection rate at the interim analysis. Rej at final: the probability of rejection at the final analysis condition on not rejecting at the interim analysis. Oracle: boundaries calculated using full data at interim. LR and TD: the proposed weighted log-rank and Tsiatis and Davidian (2024) statistics normalized using the proposed covariance estimates. BLR and BTD: the statistics normalized using the bootstrap covariance estimates. LD-Pocock and LD-OBF: Pocock and OBF boundaries obtained using a particular error spending function recommended by Lan and Demets (1983). Results are shown in percentages within 1 decimal place.

Table 7: Simulation results for 4 and 8 Treatment Strategies under Alternative Scenarios with low censoring rate around 10%,  $n = 500$

| M | Boundary  | Rejection Rate | SMART1 |     |      |     | SMART2 |     |      |     |
|---|-----------|----------------|--------|-----|------|-----|--------|-----|------|-----|
|   |           |                | Alt1   |     | Alt2 |     | Alt3   |     | Alt4 |     |
|   |           |                | LR     | TD  | LR   | TD  | LR     | TD  | LR   | TD  |
| 1 | NA        | Power          | 83     | 88  | 91   | 94  | 77     | 77  | 94   | 94  |
|   |           | Rej at interim | 39     | 46  | 47   | 58  | 31     | 33  | 55   | 51  |
|   |           | Rej at final   | 68     | 73  | 78   | 81  | 60     | 61  | 81   | 81  |
|   |           | Power          | 81     | 85  | 88   | 92  | 72     | 73  | 91   | 93  |
|   | Oracle    | $E(n)$         | 418    | 404 | 403  | 378 | 435    | 432 | 385  | 394 |
|   |           | Rej at interim | 19     | 30  | 26   | 40  | 20     | 17  | 39   | 34  |
|   |           | Rej at final   | 79     | 82  | 88   | 90  | 70     | 71  | 90   | 84  |
|   |           | Power          | 83     | 88  | 91   | 94  | 76     | 77  | 94   | 89  |
|   | OBF       | $E(n)$         | 460    | 438 | 447  | 415 | 459    | 458 | 419  | 423 |
|   |           | Rej at interim | 38     | 44  | 45   | 57  | 30     | 31  | 52   | 49  |
|   |           | Rej at final   | 67     | 72  | 76   | 81  | 58     | 58  | 80   | 80  |
|   |           | Power          | 79     | 84  | 87   | 92  | 71     | 71  | 90   | 90  |
|   |           | $E(n)$         | 420    | 407 | 405  | 381 | 438    | 436 | 390  | 397 |
|   | Pocock    | Rej at interim | 21     | 31  | 26   | 41  | 21     | 21  | 40   | 39  |
|   |           | Rej at final   | 80     | 83  | 88   | 90  | 72     | 72  | 91   | 89  |
|   |           | Power          | 84     | 88  | 91   | 94  | 78     | 78  | 94   | 94  |
|   |           | $E(n)$         | 456    | 436 | 444  | 414 | 456    | 455 | 415  | 418 |
| 2 | LD-Pocock | Rej at interim | 41     | 48  | 48   | 59  | 32     | 34  | 56   | 52  |
|   |           | Rej at final   | 65     | 71  | 75   | 80  | 58     | 58  | 79   | 79  |
|   |           | Power          | 79     | 85  | 87   | 92  | 72     | 72  | 91   | 90  |
|   |           | $E(n)$         | 414    | 400 | 400  | 376 | 433    | 428 | 383  | 391 |
|   | LD-OBF    | Rej at interim | 20     | 28  | 26   | 37  | 14     | 14  | 31   | 30  |
|   |           | Rej at final   | 79     | 83  | 88   | 91  | 73     | 73  | 91   | 90  |
|   |           | Power          | 83     | 88  | 91   | 94  | 77     | 77  | 94   | 93  |
|   |           | $E(n)$         | 459    | 442 | 446  | 423 | 470    | 470 | 436  | 438 |

M: Number of total analysis including the final. Rej at interim: rejection rate at the interim analysis. Rej at final: the probability of rejection at the final analysis condition on not rejecting at the interim analysis. Oracle: boundaries calculated using full data at interim. LR and TD: the proposed weighted log-rank and Tsiatis and Davidian (2024) statistics normalized using the proposed covariance estimates. LD-Pocock and LD-OBF: Pocock and OBF boundaries obtained using a particular error spending function recommended by Lan and Demets (1983). All results (except  $E(n)$ ) are shown in percentages rounded to integers.

Table 8: Simulation results for 2 SMART designs under Alternative Scenarios with high censoring rate around 40%

| M | Boundary  | Rejection Rate | SMART1 |     |        |     | SMART2 |     |        |     |
|---|-----------|----------------|--------|-----|--------|-----|--------|-----|--------|-----|
|   |           |                | Alt1   |     | Alt1   |     | Alt3   |     | Alt3   |     |
|   |           |                | n=500  |     | n=1000 |     | n=500  |     | n=1000 |     |
|   |           |                | LR     | TD  | LR     | TD  | LR     | TD  | LR     | TD  |
| 1 | NA        | Power          | 58     | 67  | 92     | 95  | 55     | 54  | 90     | 90  |
|   | Oracle    | Rej at interim | 21     | 30  | 50     | 57  | 21     | 22  | 48     | 48  |
|   | Pocock    | Rej at final   | 39     | 47  | 80     | 83  | 37     | 35  | 71     | 72  |
|   |           | Power          | 53     | 63  | 90     | 93  | 50     | 49  | 85     | 86  |
|   |           | E(n)           | 455    | 438 | 790    | 760 | 457    | 454 | 798    | 801 |
|   | Oracle    | Rej at interim | 8      | 15  | 28     | 38  | 12     | 12  | 32     | 32  |
|   | OBF       | Rej at final   | 54     | 61  | 89     | 91  | 47     | 48  | 83     | 85  |
|   |           | Power          | 58     | 67  | 92     | 95  | 54     | 54  | 89     | 90  |
|   |           | E(n)           | 484    | 468 | 885    | 841 | 475    | 476 | 866    | 867 |
|   | Pocock    | Rej at interim | 21     | 28  | 49     | 55  | 19     | 19  | 45     | 45  |
|   |           | Rej at final   | 38     | 45  | 78     | 82  | 34     | 34  | 69     | 70  |
|   |           | Power          | 51     | 60  | 89     | 92  | 47     | 47  | 83     | 84  |
|   |           | E(n)           | 457    | 441 | 795    | 768 | 460    | 459 | 811    | 810 |
| 2 | OBF       | Rej at interim | 8      | 15  | 29     | 39  | 13     | 13  | 34     | 35  |
|   |           | Rej at final   | 56     | 62  | 89     | 92  | 49     | 49  | 85     | 85  |
|   |           | Power          | 60     | 67  | 92     | 95  | 56     | 55  | 90     | 91  |
|   |           | E(n)           | 483    | 468 | 879    | 836 | 473    | 472 | 858    | 855 |
|   | LD-Pocock | Rej at interim | 24     | 31  | 52     | 58  | 22     | 22  | 49     | 49  |
|   |           | Rej at final   | 36     | 45  | 77     | 81  | 34     | 34  | 69     | 69  |
|   |           | Power          | 51     | 62  | 89     | 92  | 49     | 49  | 84     | 84  |
|   |           | E(n)           | 450    | 436 | 780    | 756 | 454    | 453 | 794    | 797 |
|   | LD-OBF    | Rej at interim | 8      | 14  | 28     | 36  | 9      | 8   | 24     | 25  |
|   |           | Rej at final   | 54     | 61  | 89     | 92  | 50     | 50  | 86     | 87  |
|   |           | Power          | 58     | 67  | 92     | 95  | 54     | 54  | 89     | 90  |
|   |           | E(n)           | 484    | 471 | 884    | 851 | 482    | 483 | 899    | 896 |

M: Number of total analysis including the final. Rej at interim: rejection rate at the interim analysis. Rej at final: the probability of rejection at the final analysis condition on not rejecting at the interim analysis. Oracle: boundaries calculated using full data at interim. LR and TD: the proposed weighted log-rank and Tsiatis and Davidian (2024) statistics normalized using the proposed covariance estimates. LD-Pocock and LD-OBF: Pocock and OBF boundaries obtained using a particular error spending function recommended by Lan and Demets (1983). All results (except  $E(n)$ ) are shown in percentages rounded to integers.

Table 9: Simulation results for 4 and 8 Treatment Strategies under Alternative Scenarios with  $p_\eta = 0.75$  (Censoring rates are around 10%)

| M | Boundary  | Rejection Rate | SMART1 |     |      |     | SMART2 |     |      |     |
|---|-----------|----------------|--------|-----|------|-----|--------|-----|------|-----|
|   |           |                | Alt1   |     | Alt2 |     | Alt3   |     | Alt4 |     |
|   |           |                | LR     | TD  | LR   | TD  | LR     | TD  | LR   | TD  |
| 1 | NA        | Power          | 76     | 82  | 92   | 94  | 71     | 72  | 90   | 89  |
|   | Oracle    | Rej at interim | 32     | 43  | 47   | 57  | 29     | 30  | 50   | 50  |
|   | Pocock    | Rej at final   | 58     | 63  | 77   | 81  | 51     | 50  | 73   | 74  |
|   |           | Power          | 72     | 79  | 88   | 92  | 65     | 65  | 86   | 87  |
|   |           | E(n)           | 433    | 411 | 401  | 380 | 438    | 436 | 395  | 394 |
|   | Oracle    | Rej at interim | 15     | 24  | 26   | 39  | 16     | 16  | 34   | 34  |
|   | OBF       | Rej at final   | 71     | 75  | 89   | 90  | 63     | 64  | 83   | 84  |
|   |           | Power          | 76     | 81  | 92   | 94  | 69     | 70  | 89   | 89  |
|   |           | E(n)           | 468    | 449 | 445  | 418 | 466    | 466 | 428  | 428 |
|   | Pocock    | Rej at interim | 31     | 41  | 45   | 56  | 27     | 28  | 48   | 47  |
|   |           | Rej at final   | 57     | 62  | 76   | 80  | 48     | 48  | 71   | 73  |
|   |           | Power          | 71     | 77  | 87   | 91  | 63     | 62  | 85   | 86  |
|   |           | E(n)           | 434    | 415 | 405  | 383 | 443    | 441 | 399  | 400 |
|   | OBF       | Rej at interim | 16     | 25  | 28   | 41  | 18     | 18  | 35   | 36  |
|   |           | Rej at final   | 72     | 76  | 89   | 91  | 65     | 66  | 85   | 84  |
|   |           | Power          | 77     | 82  | 92   | 95  | 71     | 72  | 90   | 90  |
|   |           | E(n)           | 466    | 447 | 442  | 415 | 463    | 462 | 425  | 424 |
|   | LD-Pocock | Rej at interim | 34     | 44  | 49   | 59  | 30     | 32  | 51   | 51  |
|   |           | Rej at final   | 55     | 61  | 74   | 79  | 49     | 47  | 71   | 72  |
|   |           | Power          | 70     | 78  | 87   | 91  | 64     | 64  | 86   | 87  |
|   |           | E(n)           | 428    | 407 | 398  | 377 | 436    | 432 | 392  | 391 |
|   | LD-OBF    | Rej at interim | 16     | 22  | 27   | 38  | 13     | 12  | 27   | 27  |
|   |           | Rej at final   | 71     | 76  | 89   | 91  | 66     | 67  | 86   | 85  |
|   |           | Power          | 76     | 81  | 92   | 94  | 70     | 71  | 90   | 89  |
|   |           | E(n)           | 467    | 453 | 444  | 422 | 474    | 474 | 443  | 444 |

M: Number of total analysis including the final. Rej at interim: rejection rate at the interim analysis. Rej at final: the probability of rejection at the final analysis condition on not rejecting at the interim analysis. Oracle: boundaries calculated using full data at interim. LR and TD: the proposed weighted log-rank and Tsiatis and Davidian (2024) statistics normalized using the proposed covariance estimates. LD-Pocock and LD-OBF: Pocock and OBF boundaries obtained using a particular error spending function recommended by Lan and Demets (1983). All results (except  $E(n)$ ) are shown in percentages rounded to integers.

Table 10: Simulation results for 4 and 8 Treatment Strategies under Alternative Scenarios with  $p_\eta = 0.75$  (Censoring rates are around 20%)

| M | Boundary  | Rejection Rate | SMART1 |     |      |     | SMART2 |     |      |     |
|---|-----------|----------------|--------|-----|------|-----|--------|-----|------|-----|
|   |           |                | Alt1   |     | Alt2 |     | Alt3   |     | Alt4 |     |
|   |           |                | LR     | TD  | LR   | TD  | LR     | TD  | LR   | TD  |
| 1 | NA        | Power          | 71     | 76  | 87   | 91  | 64     | 65  | 86   | 85  |
|   | Oracle    | Rej at interim | 30     | 37  | 40   | 52  | 26     | 15  | 47   | 47  |
|   | Pocock    | Rej at final   | 52     | 56  | 71   | 76  | 45     | 48  | 68   | 69  |
|   |           | Power          | 66     | 73  | 82   | 88  | 59     | 61  | 83   | 84  |
|   |           | E(n)           | 438    | 422 | 416  | 392 | 446    | 447 | 401  | 401 |
|   | Oracle    | Rej at interim | 13     | 20  | 21   | 33  | 15     | 15  | 29   | 31  |
|   | OBF       | Rej at final   | 66     | 70  | 83   | 86  | 56     | 58  | 80   | 79  |
|   |           | Power          | 71     | 76  | 87   | 91  | 63     | 64  | 86   | 86  |
|   |           | E(n)           | 472    | 458 | 456  | 431 | 469    | 469 | 438  | 435 |
|   | Pocock    | Rej at interim | 29     | 35  | 39   | 49  | 23     | 24  | 45   | 44  |
|   |           | Rej at final   | 50     | 55  | 70   | 74  | 43     | 45  | 66   | 67  |
|   |           | Power          | 65     | 71  | 81   | 87  | 56     | 58  | 81   | 82  |
|   |           | E(n)           | 440    | 426 | 419  | 397 | 452    | 450 | 406  | 407 |
|   | OBF       | Rej at interim | 14     | 21  | 22   | 35  | 16     | 16  | 32   | 33  |
|   |           | Rej at final   | 67     | 71  | 84   | 86  | 58     | 60  | 81   | 79  |
|   |           | Power          | 72     | 77  | 88   | 91  | 65     | 66  | 87   | 86  |
|   |           | E(n)           | 471    | 456 | 454  | 428 | 467    | 466 | 434  | 430 |
|   | LD-Pocock | Rej at interim | 31     | 39  | 43   | 53  | 27     | 27  | 48   | 48  |
|   |           | Rej at final   | 49     | 54  | 68   | 74  | 43     | 44  | 66   | 67  |
|   |           | Power          | 65     | 72  | 82   | 88  | 58     | 59  | 82   | 83  |
|   |           | E(n)           | 434    | 419 | 411  | 389 | 444    | 443 | 400  | 398 |
| 2 | LD-OBF    | Rej at interim | 13     | 19  | 21   | 31  | 11     | 10  | 23   | 23  |
|   |           | Rej at final   | 66     | 71  | 83   | 87  | 59     | 61  | 82   | 81  |
|   |           | Power          | 71     | 76  | 87   | 91  | 63     | 65  | 86   | 85  |
|   |           | E(n)           | 472    | 460 | 456  | 435 | 478    | 480 | 451  | 452 |

M: Number of total analysis including the final. Rej at interim: rejection rate at the interim analysis. Rej at final: the probability of rejection at the final analysis condition on not rejecting at the interim analysis. Oracle: boundaries calculated using full data at interim. LR and TD: the proposed weighted log-rank and Tsiatis and Davidian (2024) statistics normalized using the proposed covariance estimates. LD-Pocock and LD-OBF: Pocock and OBF boundaries obtained using a particular error spending function recommended by Lan and Demets (1983). All results (except  $E(n)$ ) are shown in percentages rounded to integers.

Table 11: Efficacy boundaries for Neuroblastoma Data

|           | LR            | TD            |
|-----------|---------------|---------------|
| Pocock    | (9.37, 9.37)  | (9.37, 9.37)  |
| OBF       | (11.07, 7.83) | (11.07, 7.83) |
| LD-Pocock | (8.85, 9.37)  | (8.92, 9.33)  |
| LD-OBF    | (12.61, 8.01) | (12.57, 7.94) |

Pocock and OBF: boundaries calculated based on covariance approximation. LD-Pocock and LD-OBF: Lan-DeMets boundaries that approximate Pocock and OBF boundaries using suitable error spending functions. LR and TD estimators are our proposed estimator and the estimator proposed in Tsiatis and Davidian (2024).
